# Supplementary material for: A modeling framework for coupling plasticity with species diffusion
Source: arXiv:2011.06652 source file (2020-11-12)
Supplement: Supplementary file 1 [file Appendix_code.tex]

\section{Computer codes}

\label{App:code}
In the following, we have provided MATLAB computer codes for coupled elastoplastic-diffusion problem. This code entails different coupling strategies and degradation models for both CG and NN formulations.
 These two formulations were discussed earlier in
Section \ref{Sec:S3_Heal_framework}.

\lstinputlisting[language=MATLAB,caption=MATLAB code
for degradation of plate with a circulate hole., label=Code:ex3,
frame=single]{Sections/Sample_code/coupled.m}
